# Supplementary material for: Interface-related magnetic and vibrational properties in Fe/MgO heterostructures from nuclear resonant spectroscopy and first-principles calculations
Source: arXiv:1911.05666 source file (2020-01-30)
Supplement: Supplementary file 1 [file Suppl-Eggert-FeMgO.pdf]

# Supplemental Material: Interface-related magnetic and vibrational properties in Fe/MgO heterostructures from nuclear resonant spectroscopy and first-principles calculations

Benedikt Eggert,[1,*] Markus E. Gruner,[1] Katharina Ollefs,[1] Ellen Schuster,[1] Nico Rothenbach,[1] Michael Y. Hu,[2] Jiyong Zhao,[2] Thomas S. Toellner,[2] Wolfgang Sturhahn,[2,3] Rossitza Pentcheva,[1] Beatriz Roldan Cuenya,[4,5] Esen E. Alp,[2] Heiko Wende,[1] and Werner Keune[1]

[1]*Faculty of Physics and Center for Nanointegration Duisburg-Essen (CENIDE), University of Duisburg-Essen, Lotharstr. 1, D-47057, Duisburg, Germany*
[2]*Advanced Photon Source, Argonne National Laboratory, Argonne, IL 60439, USA*
[3]*Division of Geophysical and Planetary Sciences, California Institute of Technology, Pasadena, CA 91125, USA*
[4]*Department of Physics, University of Central Florida, Orlando, Florida 32816, USA*
[5]*Department of Interface Science, Fritz-Haber-Institute of the Max Planck Society, 14195 Berlin, Germany*

(Dated: January 30, 2020)

In this Supplemental Material, we provide additional information concerning the sample preparation, sample characterization and the data evaluation procedure of the nuclear inelastic x-ray scattering (NRIXS) spectra.

## S1. SAMPLE PREPARATION

For the sample preparation, an ultrahigh vacuum (UHV) system with ion-getter and Ti sublimation pumps were used, providing a base pressure of $7 \cdot 10^{-10}$ mbar. For the evaporation, small pieces of metallic $^{57}$Fe (95 % isotopically enriched) and Cr were heated in home made evaporation cells with alumina crucibles, while for the evaporation of MgO, small pieces of MgO(001) crystals were used in an electron-beam heated Mo cell. The evaporation rate was monitored by two independent calibrated quartz crystal microbalances and adjusted by computer-assisted control. The configured evaporation rate was chosen to be 0.15 Å/s for $^{57}$Fe ($p_{growth} = 3 \cdot 10^{-9}$ mbar) and for MgO ($p_{growth} = 2 \cdot 10^{-8}$ mbar), while the Cr ($p_{growth} = 3 \cdot 10^{-9}$ mbar) buffer and capping layer were evaporated with a rate of 0.1 Å/s. Under these conditions polycrystalline $\left[^{57}\mathrm{Fe/MgO}\right]_{15.5}$ multilayers, with Fe thicknesses $t_{Fe}$= 1.5 nm, 4 nm and 8 nm and with a MgO-thickness $t_{MgO}$ of 4 nm were grown at room temperature on naturally oxidized Si(001) substrates covered with a 4-nm thick Cr buffer layer, while a fourth sample had thinner layers with $t_{Fe}$=1 nm and $t_{MgO}$ = 1 nm. All samples were capped with 5 nm Cr for protection. For the following discussion, the individual Fe and MgO layer thickness are expressed in units of atomic Fe(001) and MgO(001) geometrical monolayers. Therefore, one monolayer Fe (MgO) corresponds to a thickness of 1.45 Å(2.1 Å). Using this conversion, our samples have a $^{57}$Fe thickness $t_{Fe}$ of 55, 28 and 10 ML with a MgO thickness $t_{MgO}$ of 19 ML and the fourth samples consists of $t_{Fe}$=7 ML and $t_{MgO}$=5 ML.

* corresponding author: Benedikt.Eggert@uni-due.de

## S2. STRUCTURAL CHARACTERISATION

For the investigation of the crystalline nature of the prepared multilayer structure, we performed x-ray diffraction (XRD) measurements at room temperature using Cu $K_\alpha$ radiation in a Bragg-Brentano geometry, using a Philips x-ray diffractometer (PW1730) equipped with a graphite monochromator. From the diffractogram, shown in Figure S1(a), one can see for the sample with a $^{57}$Fe-layer thickness of 55 ML peaks for MgO(200), Fe(110), Fe(211), Fe(200) and the substrate Si(100) peak. Fig. S1(b) displays a zoom of the Fe(110) peak, where the MgO(200) peak appears as a weak shoulder near 42.5°. With decreasing $^{57}$Fe-layer thickness, the MgO and Fe peaks broaden and, therefore, the intensity decreases. This effect is due to the decreasing size of the crystallites. The average crystallite size was estimated from the peak width using the Scherrer equation. The lattice parameters $a_{Fe}$ and $a_{MgO}$ and grain size $d_{Fe}$ and $d_{MgO}$ obtained from Fig. S1(a) for the investigated multilayer samples are presented in Table S1 for $t_{Fe}$= 55, 28, 10 and 7 ML. The obtained lattice constants are in good agreement with bulk bcc Fe (2.86 Å) and bulk MgO (4.217 Å), respectively. A precise determination of the Fe lattice constant is difficult, due to the overlap of the Fe(110) and Cr(110) Bragg peaks.

## S3. MÖSSBAUER SPECTROSCOPY

Zero field Conversion Electron Mössbauer spectroscopy was performed at room temperature (RT) to further analyze the magnetic structure and phase composition (Figure S2). The obtained spectra were analyzed in a similar way, as it was discussed in the main text (Section IV.A) using a hyperfine field distribution $p\left(B_{hf}\right)$ (right side of

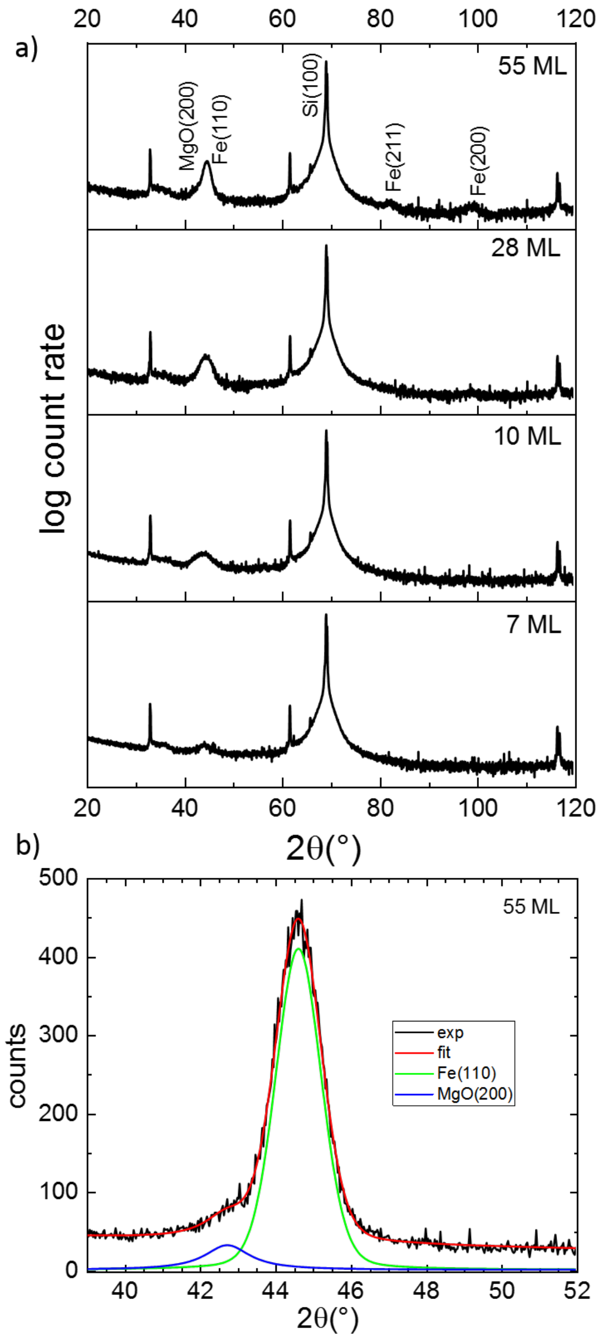


FIG. S1. a) X-ray diffraction (XRD) pattern (Cu-$K_\alpha$-radiation, $\lambda = 1.5406$ Å) of the [Fe/MgO]-multilayers with $t_{Fe}$=55, 28, 10 and 7 ML. The position of the Fe, MgO and Si peaks are labeled. The additional peaks at 33°, 61.7°, 65.9° and 116.5° are due to $\frac{1}{2}$Cu $K_\alpha$ Si(100), Cu $K_\beta$ Si(100), W $L_\alpha$ Si(100) and Cu $K_\alpha$ (200) Bragg reflexes.
b) Detailed illustration of the overlap between Fe(110) and MgO(200) between 40° and 48° for the sample with $t_{Fe}$=55 ML.

TABLE S1. Lattice constant $a_{Fe}$ and $a_{MgO}$ and grain size $d_{Fe}$ and $d_{MgO}$ of Fe and MgO for the investigated [Fe/MgO]-multilayer system obtained by Rietveld analysis from XRD measurements performed at RT. The obtained lattice constants are in relatively good agreement with those of bulk bcc Fe (2.86 Å) and bulk MgO (4.217 Å), respectively.

| $t_{Fe}$ Fe ML | $a_{Fe}$ (Å) | $d_{Fe}$ (Å) | $a_{MgO}$ (Å) | $d_{MgO}$ (Å) |
|---|---|---|---|---|
| 55 | 2.874 ± 0.017 | 60.4 ± 0.4 | 4.235 ± 0.384 | 59.4±4.8 |
| 28 | 2.883 ± 0.088 | 35.4 ± 0.6 | 4.253 ± 0.340 | 49.8±3.0 |
| 10 | 2.914 ± 0.200 | 24.7 ± 0.9 | 4.249 ± 0.093 | 68.7±7.9 |
| 7 | 2.892 ± 0.333 | 36.8 ± 3.0 | 4.296 ± 0.078 | 22.4±8.9 |

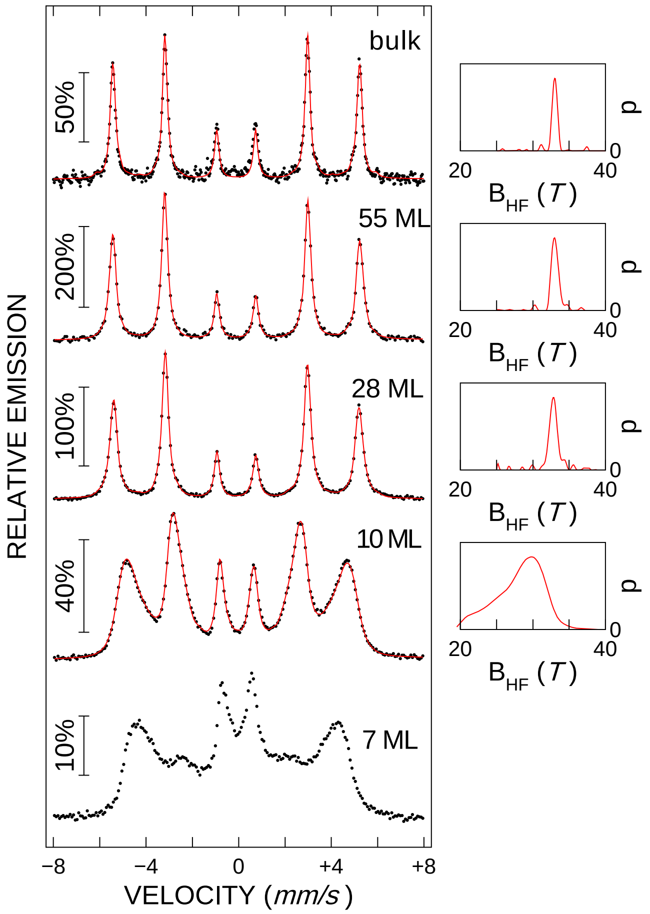


FIG. S2. Result of zero-field CEMS measurements at $T$ = 300 K for bulk bcc-Fe (top) and [Fe/MgO] multilayers with varying Fe thicknesses $t_{Fe}$ of 55, 28, 10 and 7 monolayers (ML). Black dots: experimental data; red lines: least-squares fitted curves using the corresponding hyperfine-field distributions $p(B_{hf})$ obtained from the fittings, which is shown in each case on the right-hand side. For the 10-ML sample, beginning thermal magnetic relaxation phenomena are evident, as inferred from the asymmetric line shape and line broadening. For the 7 ML sample, even faster thermal relaxation is evident, where, in addition to the asymmetric lineshape and large line broadening, a central spectral feature ("doublet") appears. Therefore, the spectrum of the 7 ML sample is not described by a static $p(B_{hf})$ distribution.

TABLE S2. Mössbauer parameters for the investigated samples obtained from least-squares fitting of the spectra seen in Figure S2 based on the corresponding distribution of hyperfine fields, $p\,(B_{hf})$ for the different samples with varying Fe-layer thickness $t_{Fe}$. $\langle\delta_{iso}\rangle$ is the average isomer shift relative to bulk bcc-Fe at room temperature, $\Gamma$ describes the intrinsic linewidth (FWHM) of the used sextets in the distribution, $\langle B_{hf}\rangle$ refers to the average magnetic hyperfine field between 25 T and 45 T, $\sigma_{B_{hf}}$ is the standard deviation of the obtained distribution, $A_{2,3}$ is obtained by the intensity ratio of lines 2 and 3, $\langle\Theta\rangle$ describes the average angle between Fe spin direction and the incident $\gamma$-ray direction determined from the $A_{2,3}$-ratio shown in equation (1) of the main text.

| $t_{Fe}$ | $\langle\delta_{iso}\rangle$ (mm/s) | $\Gamma$ (mm/s) | $\langle B_{hf}\rangle$ (T) | $\sigma_{B_{hf}}$ (T) | $A_{2,3}$ | $\langle\Theta\rangle$ (°) |
|---|---|---|---|---|---|---|
| bulk | 0.00(1) | 0.238(4) | 33.0(4) | 1.4 | 3.34(5) | 72.5 |
| 55 ML | 0.01(9) | 0.265(2) | 33.0(5) | 1.2 | 3.66(4) | 77.7 |
| 28 ML | 0.01(7) | 0.272(1) | 32.7(6) | 1.6 | 3.78(2) | 80.1 |
| 10 ML | 0.02(1) | 0.336(2) | 26.5(2) | 6.0 | 2.78(1) | 64.8 |

Fig S2), while the obtained fitting parameters are shown in Table S2. In comparison with the results discussed in the main text, for the bcc-Fe bulk sample and the multilayer samples with a Fe layer thickness $t_{Fe}$ of 55 and 28 ML, similar trends of the hyperfine parameters are present, while the changes of the magnitude of the average hyperfine field $\langle B_{hf}\rangle$ and average isomer shift $\langle\delta_{iso}\rangle$ can be explained by the different measurement temperature. At room temperature, the Fe spin orientation is preferred in the film plane, as it is evident from $\langle\Theta\rangle$. In the following, we want to focus on two aspects:

First, we want to emphasize the absence of a secondary iron oxide phase, e.g. $FeO_{1-x}$ (Wustite), located at the Fe/MgO interface. At room temperature Wustite is characterized by a paramagnetic asymmetric feature with an isomer shift $\delta_{iso}$ of 1 mm/s[S1]. This statement can be made for all the present samples since all contributions show an average isomer shift $\langle\delta_{iso}\rangle$ close to 0 mm/s (reference value of bulk bcc-Fe). Furthermore, for the multilayer sample with an Fe layer thickness $t_{Fe}$ of 10 and 7 ML a thermal magnetic relaxation process occurs. For the 10 ML sample, this thermal relaxation process is indicated by the reduced average hyperfine field $\langle B_{hf}\rangle$, and the asymmetric spectral line shape. In the hyperfine field distribution $p\,(B_{hf})$, this magnetic thermal relaxation process is illustrated by an asymmetric distribution with a broad extension towards lower fields. This relaxation process leads to the increased intrinsic linewidth $\Gamma$ and deviation $\sigma_{B_{hf}}$ for this sample. For the 7 ML sample, this thermal relaxation process is enhanced. Here a central spectral feature ("doublet") is present, in addition to an asymmetry of the emission intensity at - 1.6 and 1.6 mm/s. Similar effects have been observed for example for ultrathin $^{57}Fe(100)$ films grown on Ag(100)[S2], indicating island growth of the $^{57}Fe$ layers for the thinnest studied sample.

## S4. MAGNETIC CHARACTERIZATION

In addition to the 80 K magnetometry measurements presented in the main text, measurements at 4.3 K have been performed (see Figure S3. All samples show similar saturation magnetisation $M_s$ like bcc-Fe with a deviation up to ± 5% to the known literature value at 0 K[S3] $\left(M_s^{\text{bulk}} = 1747\,\text{emu/cm}^3\right)$. In comparison to the 80 K measurements an increased coercivity field is present at T = 4.3 K, while the ouf-of-plane coercivity is larger compared to the in-plane one. These values are shown in Table S3.

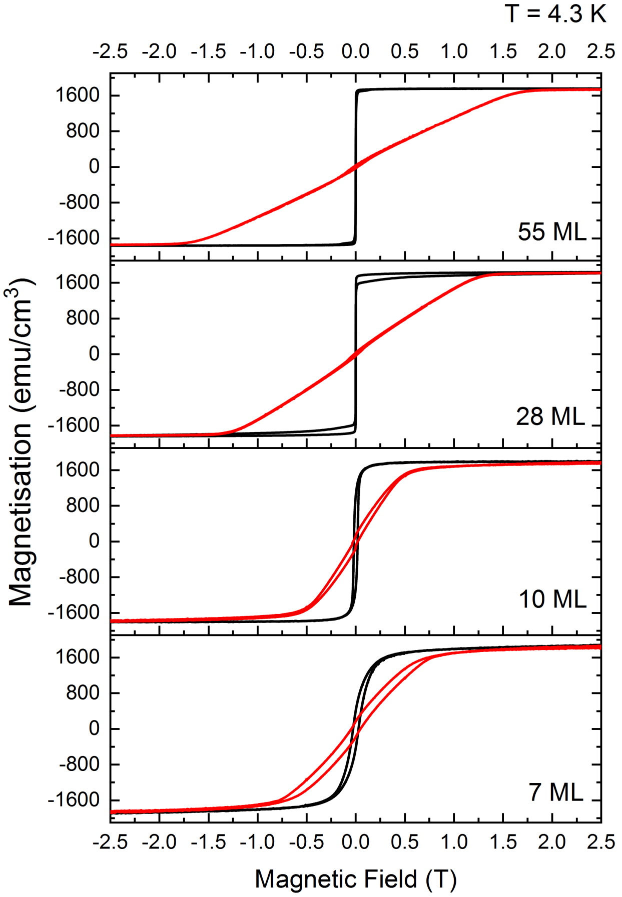


FIG. S3. Field dependent magnetization curves measured for different Fe thicknesses for in-plane and out-of-plane geometry. Measurements have been performed at T = 4.2 K.

TABLE S3. Magnetic properties obtained from hysteresis curves performed at T=4.3 K for varying Fe thickness $t_{Fe}$, where $M_s$ describes the saturation magnetization, $H_k$ the anisotropy field and $H_c$ the coercivity field.

| $t_{Fe}$ Fe ML | $M_s$ (emu/cm$^3$) | $\mu_0 H_k$ (T) | $\mu_0 H_c$ (mT) in-plane | out-of-plane |
|---|---|---|---|---|
| 55 | 1770 | 1.675 | <2 | 15.5 |
| 28 | 1832 | 1.285 | <2 | 17 |
| 10 | 1805 | 0.541 | 19 | 20 |
| 7 | 1746 | 0.69 | 30 | 46 |

## S5. NUCLEAR RESONANT INELASTIC X-RAY SCATTERING

The Fe-specific (Fe-partial) vibrational density of states (VDOS, $g(E)$) have been extracted from the raw data utilizing the PHOENIX software [S4, S5].

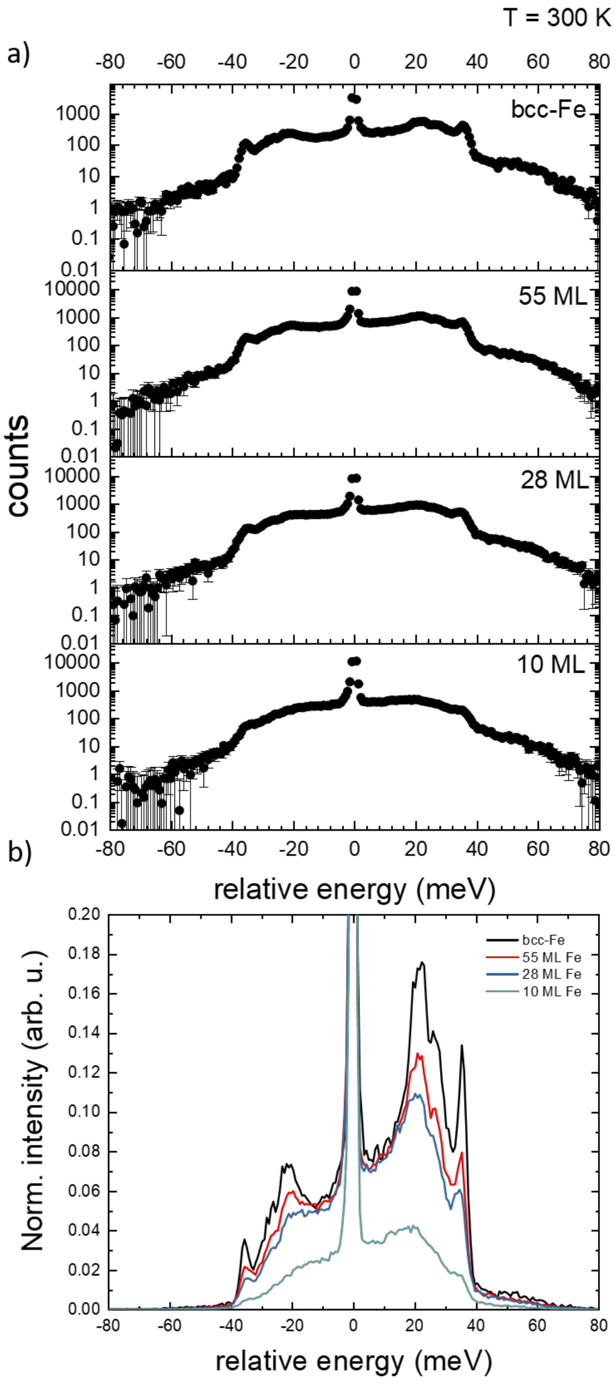


FIG. S4. NRIXS spectra (raw data) of bcc-Fe foil and the [Fe/MgO]-multilayers with $t_{Fe}$=55, 28, and 10 ML (black dots) and the respective least-squares fits (red lines) obtained from the PHOENIX software. Measurements have been performed at room temperature. The spectrum of the bcc-Fe reference has been taken from Ref. [S6].

In Figure S4(a), the raw spectra for the present multilayer samples (and for bulk bcc Fe for comparison [S6]) are shown in an energy range up to E = ± 80 meV ($= E_\gamma - E_0$) around the Mössbauer resonance ($E_0$ = 14.412 keV). For a better comparison of the spectral changes for the different samples, the spectra are shown in Figure S4(b) normalized to the elastic (Mössbauer) peak intensity. From this representation one can, for example, observe the reduction of the longitudinal acoustic phonon mode below 40 meV with decreasing Fe-layer thickness. Employing the PHOENIX software[S4, S5], the raw NRIXS spectra (Fig. S4) were normalized according to Lipkin's sum rules [S7], and the central elastic peak (= resolution function of 1.3 meV FWHM) was removed from the data. The result represents the normalized phonon excitation probability shown in Figure S5. Due to the subtraction of the elastic peak, the low energy data in the range E between about ±5 meV are physically meaningless. In Fig. S5, a reduction of the longitudinal acoustic phonon peak near +40 meV with

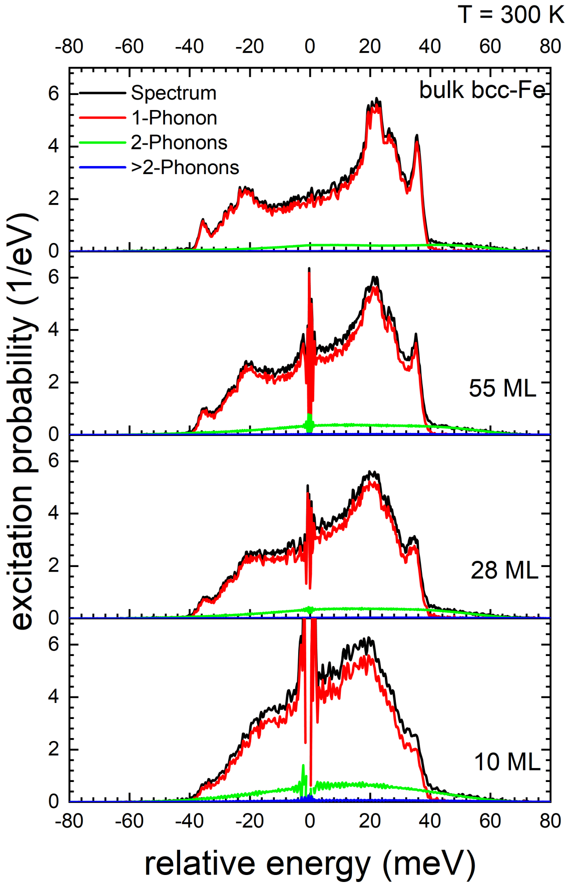


FIG. S5. Phonon excitation probability of the bcc-Fe reference foil and the different [Fe/MgO] multilayers obtained from Fig. S4 after proper normalization according to Lipkin's sum rules [S7] and subtraction of the elastic peak (= resolution function) at zero energy transfer. The results were obtained from the PHOENIX software. One-phonon contribution: red lines; two-phonon contribution: green lines; multiphonon contribution: blue lines. Experimental data (black lines) were obtained at room temperature

The Fe-specific VDOS, $g(E)$, for the three multilayer samples and for bulk bcc-Fe (reference) obtained from the data in Fig. S5 via the PHOENIX software are displayed in Figure 4 of the main text of this manuscript. From Figure S6, it is possible to determine the average Debye sound velocity $\langle v_D \rangle$, as discussed in the main text. For a general description of the derivation of $\langle v_D \rangle$ from NRIXS, we refer the reader to the work of Achterhold et al. [S8], Hu et al. [S9] and Morrison et al [S10]. In this work, the average Debye sound velocity $\langle v_D \rangle$ was determined by the method discussed by Morrison et al. [S10] with the empirical power law

$$v(E) = \langle v_D \rangle \left( 1 - \left( \frac{E}{A_1} \right)^4 \right), \tag{S1}$$

where $A_1$ is a fit parameter and represents the effective curvature of the phonon dispersion curve. $v(E)$ can be obtained by conversion of Equation (3) of the main text to

$$v(E) = \left( \frac{m}{2\pi^2 \hbar \rho} \frac{1}{g(E)} E^2 \right)^{1/3}, \tag{S2}$$

where the low energy part of the VDOS is considered for the evaluation of $\langle v_D \rangle$. The increase of the low energy part of $g(E)/E^2$ with decreasing Fe layer thickness $t_{Fe}$, clearly evident in Fig. S6, indicates elastic softening and a reduction of the average sound velocity $\langle v_D \rangle$ with decreasing $t_{Fe}$ in the multilayers.

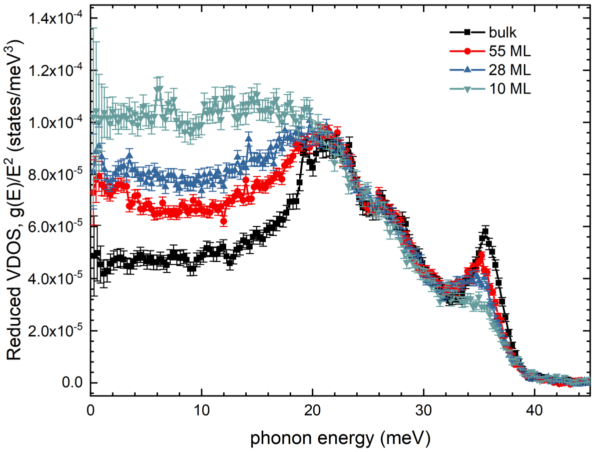


FIG. S6. Reduced Fe-partial VDOS, $g(E)/E^2$, obtained from NRIXS for a bcc-Fe foil and for the different [Fe/MgO] multilayers with varying Fe thicknesses $t_{Fe}$. The $g(E)$ data were obtained using the PHOENIX software. The data below about 5 meV are physically meaningless because of the uncertainties induced by the subtraction of the elastic peak.


[S1] C. A. McCammon and D. C. Price, Mössbauer spectra of fe x o (x0.95), Physics and Chemistry of Minerals **11**, 250 (1985).

[S2] N. C. Koon, B. T. Jonker, F. A. Volkening, J. J. Krebs, and G. A. Prinz, Direct evidence for perpendicular spin orientations and enhanced hyperfine fields in ultrathin fe(100) films on ag(100), Phys. Rev. Lett. **59**, 2463 (1987).

[S3] H. Danan, A. Herr, and A. J. P. Meyer, New determinations of the saturation magnetization of nickel and iron, Journal of Applied Physics **39**, 669 (1968).

[S4] W. Sturhahn, CONUSS and PHOENIX: Evaluation of nuclear resonant scattering data, Hyperfine Interactions **125**, 149 (2000).

[S5] W. Sturhahn, Nuclear resonant spectroscopy, Journal of Physics: Condensed Matter **16**, S497 (2004).

[S6] T. S. Toellner, M. Y. Hu, W. Sturhahn, K. Quast, and E. E. Alp, Inelastic nuclear resonant scattering with sub-meV energy resolution, Applied Physics Letters **71**, 2112 (1997).

[S7] H. J. Lipkin, Mössbauer sum rules for use with synchrotron sources, Physical Review B **52**, 10073 (1995).

[S8] K. Achterhold, C. Keppler, A. Ostermann, U. van Bürck, W. Sturhahn, E. E. Alp, and F. G. Parak, Vibrational dynamics of myoglobin determined by the phonon-assisted Mössbauer effect, Physical Review E **65**, 051916 (2002).

[S9] M. Y. Hu, W. Sturhahn, T. S. Toellner, P. D. Mannheim, D. E. Brown, J. Zhao, and E. E. Alp, Measuring velocity of sound with nuclear resonant inelastic x-ray scattering, Physical Review B **67**, 094304 (2003).

[S10] R. A. Morrison, J. M. Jackson, W. Sturhahn, J. Zhao, and T. S. Toellner, High pressure thermoelasticity and sound velocities of fe-ni-si alloys, Physics of the Earth and Planetary Interiors **294**, 106268 (2019).
